# Supplementary material for: Ising-Based Louvain Method: Clustering Large Graphs with Specialized Hardware
Source: arXiv:2012.11391 source file (2020-12-06)
Supplement: Supplementary file 1 [file appendix.tex]

% \section{Appendices}
% \label{sec:appendix}
% Appendices are material that can be read, and include lemmas, formulas, proofs, and tables that are not critical to the reading and understanding of the paper. 
% Appendices should be \textbf{uploaded as supplementary material} when submitting the paper for review.
% Upon acceptance, the appendices come after the references, as shown here.
\appendix
\subsection{Derivation of Equation \ref{eq:25}} \label{sec:appendix}
\noindent We can expand the right-hand-side (RHS) of Equation \ref{eq:16} as follows:
\begin{equation} \label{eq:17}
         {\boldsymbol{x}}^T \Big( \frac{1}{2m}\mathbbm{k} \mathbbm{k}^T  - {\boldsymbol{A}}\Big){\boldsymbol{x}} = \frac{1}{2m} {\boldsymbol{x}}^T \mathbbm{k} \mathbbm{k}^T {\boldsymbol{x}} - {\boldsymbol{x}}^T {\boldsymbol{A}} {\boldsymbol{x}}
\end{equation}

The first term on the RHS of Equation \ref{eq:17} can then be simplified as follows:
\begin{multline}
\begin{aligned}
         &{\boldsymbol{x}}^T \mathbbm{k} \mathbbm{k}^T {\boldsymbol{x}} = \sum_{i} \sum_{j} x_i k_i k_j x_j = \sum_{i} x_i k_i \sum_{j} k_j x_j
         \\&= \sum_{i \in S} x_i k_i \sum_{j} k_j x_j + \sum_{i \in C} x_i k_i \sum_{j} k_j x_j + \sum_{i \in \bar{C}} x_i k_i \sum_{j} k_j x_j
         \\&= \sum_{i \in S} x_i k_i \sum_{j \in S} k_j x_j + \sum_{i \in S} x_i k_i \sum_{j \in C} k_j x_j + \sum_{i \in S} x_i k_i \sum_{j \in \bar{C}} k_j x_j + \sum_{i \in C} x_i k_i \sum_{j \in S} k_j x_j
         \\&+ \sum_{i \in C} x_i k_i \sum_{j \in C} k_j x_j + \sum_{i \in C} x_i k_i \sum_{j \in \bar{C}} k_j x_j + \sum_{i \in \bar{C}} x_i k_i \sum_{j \in S} k_j x_j + \sum_{i \in \bar{C}} x_i k_i \sum_{j \in C} k_j x_j
         \\&+ \sum_{i \in \bar{C}} x_i k_i \sum_{j \in \bar{C}} k_j x_j
\end{aligned} \\\label{eq:18}
\end{multline}
\noindent here, $S$ is the set of $S$ free nodes, $C$ is the candidate cluster for the free nodes, and $\bar{C}$ is a set containing the rest of the nodes in the graph, $i.e.$ not included in $C$ or $S$. Based on these definitions, $S$, $C$, and $\bar{C}$ are mutually exclusive.

\noindent The last expression on the RHS of Equation \ref{eq:18} can be further simplified as follows:
\begin{multline} 
\begin{aligned}
    &{\boldsymbol{x}}^T \mathbbm{k} \mathbbm{k}^T {\boldsymbol{x}}
    \\&= \sum_{i \in S} x_i k_i \sum_{j \in S} k_j x_j + \sum_{i \in S} x_i k_i \sum_{j \in C} k_j \times 1 + \sum_{i \in S} x_i k_i \sum_{j \in \bar{C}} k_j \times 0
    \\&+ \sum_{i \in C} 1 \times k_i \sum_{j \in S} k_j x_j + \sum_{i \in C} 1 \times k_i \sum_{j \in C} k_j \times 1 + \sum_{i \in C} 1 \times k_i \sum_{j \in \bar{C}} k_j \times 0
    \\&+ \sum_{i \in \bar{C}} 0 \times k_i \sum_{j \in S} k_j x_j + \sum_{i \in \bar{C}} 0 \times k_i \sum_{j \in C} k_j \times 1 + \sum_{i \in \bar{C}} 0 \times k_i \sum_{j \in \bar{C}} k_j \times 0
    \\&=
    \sum_{i \in S} x_i k_i \sum_{j \in S} k_j x_j + \sum_{i \in S} x_i k_i \sum_{j \in C} k_j + \sum_{i \in C} k_i \sum_{j \in S} k_j x_j + \sum_{i \in C} k_i \sum_{j \in C} k_j
\end{aligned} \label{eq:19}
\end{multline}

\noindent where in the last expression, the second and third terms are the same (we only need to swap $i$ and $j$), so we have:
\begin{equation} \label{eq:20}
    {\boldsymbol{x}}^T \mathbbm{k} \mathbbm{k}^T {\boldsymbol{x}} = \sum_{i \in S} x_i k_i \sum_{j \in S} k_j x_j + 2\sum_{i \in S} x_i k_i \sum_{j \in C} k_j + \sum_{i \in C} k_i \sum_{j \in C} k_j
\end{equation} %\\= (\sum_{i \in S} x_i k_i + \sum_{i \in C} k_i)^2

We can also expand the last term on the RHS of Equation \ref{eq:17} as follows:
\begin{multline} 
\begin{aligned}
    &{\boldsymbol{x}}^T {\boldsymbol{A}} {\boldsymbol{x}} = \sum_{i} \sum_{j} x_i A_{i,j} x_j = \sum_{i \in S} \sum_{j \in S} x_i A_{i,j} x_j + \sum_{i \in C} \sum_{j \in S} x_i A_{i,j} x_j
    \\&+ \sum_{i \in \bar{C}} \sum_{j \in S} x_i A_{i,j} x_j + \sum_{i \in S} \sum_{j \in C} x_i A_{i,j} x_j + \sum_{i \in C} \sum_{j \in C} x_i A_{i,j} x_j + \sum_{i \in \bar{C}} \sum_{j \in C} x_i A_{i,j} x_j
    \\&+ \sum_{i \in S} \sum_{j \in \bar{C}} x_i A_{i,j} x_j + \sum_{i \in C} \sum_{j \in \bar{C}} x_i A_{i,j} x_j + \sum_{i \in \bar{C}} \sum_{j \in \bar{C}} x_i A_{i,j} x_j
\end{aligned}\\ \label{eq:21}
\end{multline}

The last expression in Equation \ref{eq:21} can be further simplified similar to what was done for \ref{eq:19}:
\begin{multline} 
\begin{aligned}
    &{\boldsymbol{x}}^T {\boldsymbol{A}} {\boldsymbol{x}}
    \\&= \sum_{i \in S} \sum_{j \in S} x_i A_{i,j} x_j + \sum_{i \in C} \sum_{j \in S} 1 \times A_{i,j} x_j + \sum_{i \in \bar{C}} \sum_{j \in S} 0 \times A_{i,j} x_j + \sum_{i \in S} \sum_{j \in C} x_i A_{i,j} \times 1
    \\&+ \sum_{i \in C} \sum_{j \in C} 1 \times A_{i,j} \times 1
    + \sum_{i \in \bar{C}} \sum_{j \in C} 0 \times A_{i,j} \times 1 + \sum_{i \in S} \sum_{j \in \bar{C}} x_i A_{i,j} \times 0
    \\&+ \sum_{i \in C} \sum_{j \in \bar{C}} 1 \times A_{i,j} \times 0 + \sum_{i \in \bar{C}} \sum_{j \in \bar{C}} 0 \times A_{i,j} \times 0 = \sum_{i \in S} \sum_{j \in S} x_i A_{i,j} x_j
    + \sum_{i \in C} \sum_{j \in S} A_{i,j} x_j
    \\&+ \sum_{i \in S} \sum_{j \in C} x_i A_{i,j}
    + \sum_{i \in C} \sum_{j \in C} A_{i,j}
\end{aligned}\\ \label{eq:22}
\end{multline}

Again, the second and third terms in the final expression in Equation \ref{eq:22} become the same after swapping $i$ and $j$ in one of them and considering that ${\boldsymbol{A}}$ is a symmetric matrix ($i.e.$ $A_{i,j} = A_{j,i}$).

\begin{equation} \label{eq:23}
    {\boldsymbol{x}}^T {\boldsymbol{A}} {\boldsymbol{x}} = \sum_{i \in S} \sum_{j \in S} x_i A_{i,j} x_j
    + 2\sum_{i \in S} \sum_{j \in C} x_i A_{i,j} + \sum_{i \in C} \sum_{j \in C} A_{i,j} 
\end{equation} % = \textbf{x$_S$}^T \textbf{A$_S$} \textbf{x$_S$}    \\&+ 2\sum_{i \in S} \sum_{j \in C} x_i A_{i,j}  + Deg(C)

\noindent The last term in the RHS expression is constant, so it can be dropped when writing the objective function of the optimization. %can also be written as $2 |E_{C}|$.\\

Inserting the results of Equations \ref{eq:20} and \ref{eq:23} into Equation \ref{eq:17} and dropping the constant terms results in
\begin{multline} \label{eq:24}
\begin{aligned}
         &{\boldsymbol{x}}^T \Big( \frac{1}{2m}\mathbbm{k} \mathbbm{k}^T  - {\boldsymbol{A}}\Big){\boldsymbol{x}} = \frac{1}{2m} {\boldsymbol{x}}^T \mathbbm{k} \mathbbm{k}^T {\boldsymbol{x}} - {\boldsymbol{x}}^T {\boldsymbol{A}} {\boldsymbol{x}}
         \\&\equiv \frac{1}{2m} \Big( \sum_{i \in S} x_i k_i \sum_{j \in S} k_j x_j + 2\sum_{i \in S} x_i k_i \sum_{j \in C} k_j \Big) - \sum_{i \in S} \sum_{j \in S} x_i A_{i,j} x_j
         \\&- 2\sum_{i \in S} \sum_{j \in C} x_i A_{i,j}
\end{aligned} 
\end{multline}
